# Supplementary material for: The effect of boron incorporation on leakage and wake-up in ferroelectric Al_{1-x}Sc_xN
Source: arXiv:2503.08399 source file (2025-03-11)
Supplement: Supplementary file 1 [file JAP_supplement.pdf]

Supplemental Section for :  
The effect of boron incorporation on leakage and wake-up in  
ferroelectric AlScN

Maiké Gremmel,<sup>1,\*</sup> Chandrashekhhar Prakash Savant,<sup>2</sup> Debaditya  
Bhattacharya,<sup>3</sup> Georg Schönweger,<sup>1, 4</sup> Debdeep Jena,<sup>2, 3, 5</sup> and Simon Fichtner<sup>1, 4</sup>

<sup>1</sup> Institute of Material Science, Kiel University, Germany

<sup>2</sup> Department of Materials Science and Engineering, Cornell University, United States

<sup>3</sup> School of Electrical and Computer Engineering, Cornell University, United States

<sup>4</sup> Fraunhofer Institute for Silicon Technology (ISIT), Germany

<sup>5</sup> Kavli Institute at Cornell for Nanoscale Science, Cornell University, United States

(Dated: February 17, 2025)

Ellipsometry measurements for Bandgap estimation:

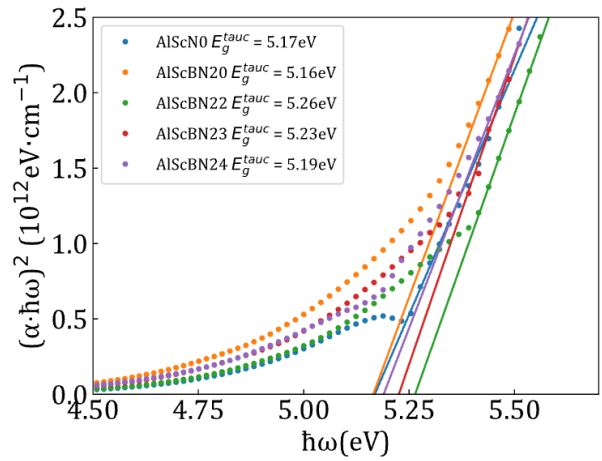

**Figure S1:** Linear Fit in linear Regime of the Ellipsometry data with the intersect of the fit with x as the estimated Bandgap Energy

The bandgap of the AlScBN films was determined via a Tauc fit from Ellipsometry. All 16 elements of the Mueller matrix were obtained with a J.A. Woolam RC2 Ellipsometer at 5 separate positions on each sample. The spectral range collected was 193 nm – 1690 nm and the angles of incidence were between 45 degrees and 75 degrees with steps of 5 degrees. The optical bandgap extraction procedure was adopted from Baeumler et al [1]. The data was fit to a KK-Enforced B-Spline model for the dielectric function for each measurement independently. We use the relation  $\alpha(\hbar\omega) = \frac{4\pi\text{Im}(\sqrt{\epsilon(\hbar\omega)})}{\lambda}$  to find the absorption coefficient. We then use Tauc's procedure to extract the bandgap from the relation  $E_g \propto (\alpha \cdot \hbar\omega)^2$ . [2]

### XRD measurements to determine lattice parameters and crystal quality:

For the calculation of the lattice parameters for the wurtzite structure two diffraction peaks were measured -(0002)/(002) and (0-115)/(0-15). For 0002 a normal  $\theta - 2\theta$  scan was performed and by knowing the angle of the peak  $2\theta$ , and the wavelength  $\lambda$ , the lattice spacing  $d$  can be calculated by Bragg's law:

$$2d = \frac{\lambda}{\sin(\theta)} \quad (1)$$

Further, the lattice spacing for hexagonal structures can be described by the lattice parameters  $a, b, c$  and the miller indices  $h, k, l$  as follows, because  $a = b$  :

$$\frac{1}{d^2} = \frac{4}{3} \frac{h^2 + hk + k^2}{a^2} + \frac{l^2}{c^2} \quad (2)$$

By choosing the reflection of 002, the first fractions become 0, and the equation can be rewritten as

$$c = 2 \cdot d \quad (002) \quad (3)$$

To calculate  $a$ , an asymmetric  $2\theta/\omega$  measurement was performed to determine the (0-15) position. Rewriting equation 2 leads to:

$$a = \sqrt{\frac{\frac{4}{3}d^2}{1 - \frac{l^2}{c^2}}} \quad (4)$$

## Electrical measurements to determine ferroelectric properties

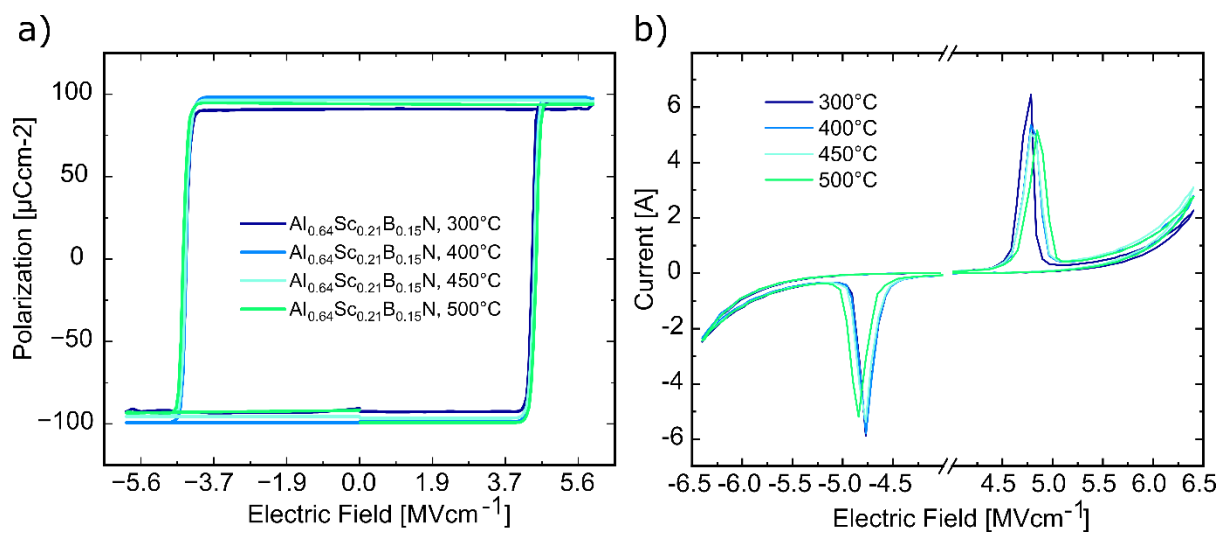

**Figure S3:** a)  $J$ - $E$  and b)  $P$ - $E$  measurement of  $\text{Al}_{0.64}\text{Sc}_{0.21}\text{B}_{0.15}\text{N}$  films after 10 cycles deposited at different temperatures.  $E_C$ ,  $P_r$  as well as leakage is similar for all samples.

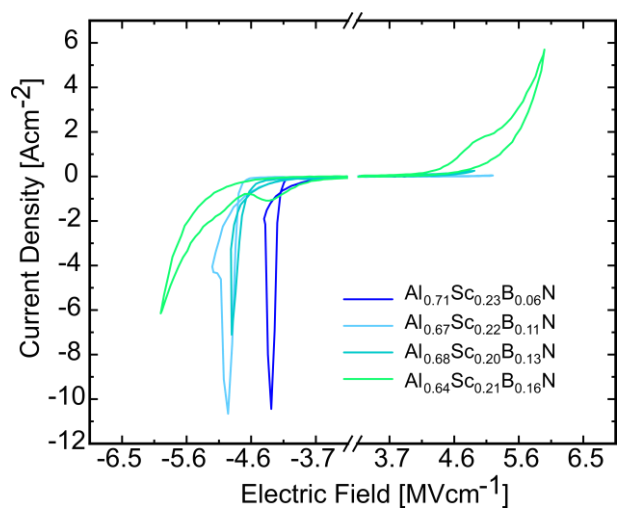

**Figure S4:**  $J$ - $E$  measurement on pristine samples of different boron concentration. While 6-13% don't show a displacement peak for a positive voltage train, 16% exhibits a broad leakage tail with a displacement peak. From the Setup of the aixACCT a positive voltage corresponds to N-polarity while a negative electric field corresponds to M-polarity. Therefore the films grow N-polar except for 16%.

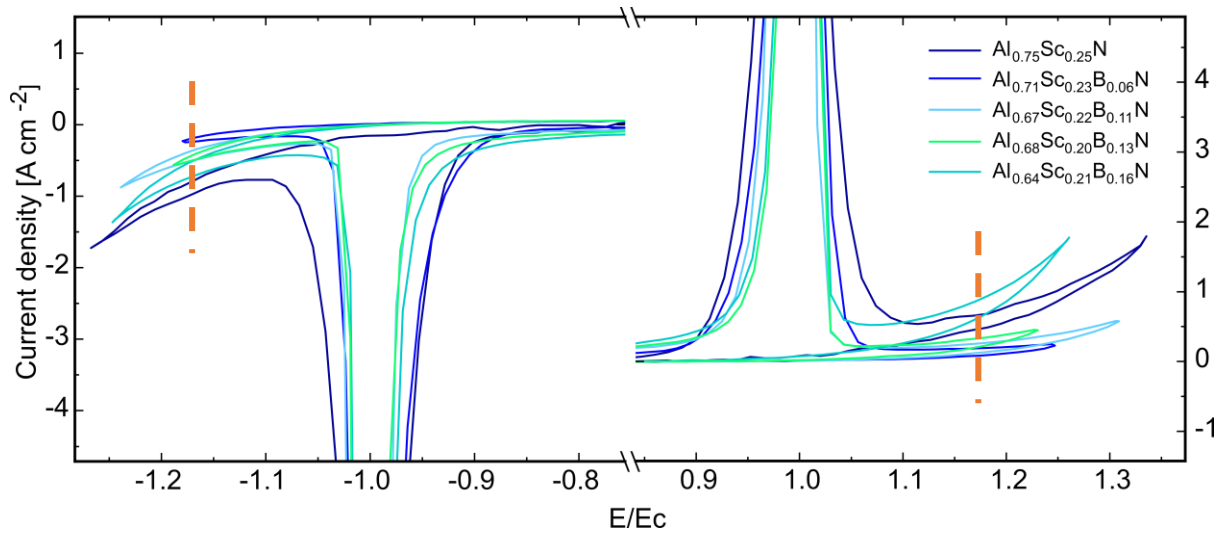

**Figure S5:**  $J$ - $E$  measurement of films with different Boron concentrations normalised to  $E_c$  for investigations of leakage. Leakage was extracted at the red line from the decreasing path of current density.

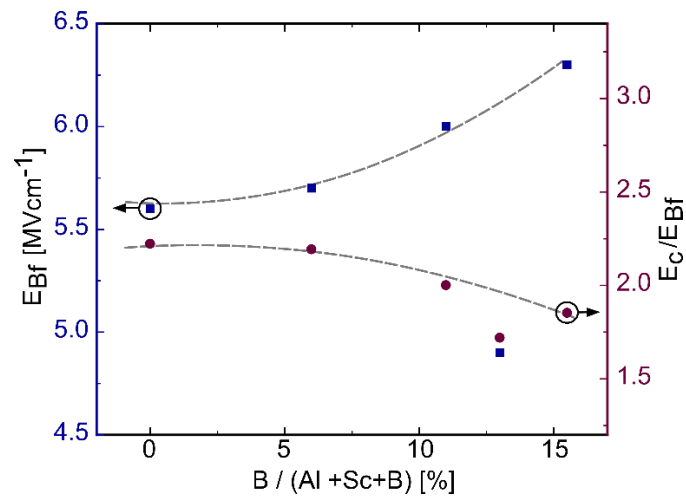

**Figure S6:** Breakdown field  $E_{Bf}$  measured by Capacitance vs Voltage measurements. Voltage range is increased until the capacitor breaks. This is repeated multiple time on different structures to confirm  $E_{Bf}$

### Frequency extrapolation of AIBN film

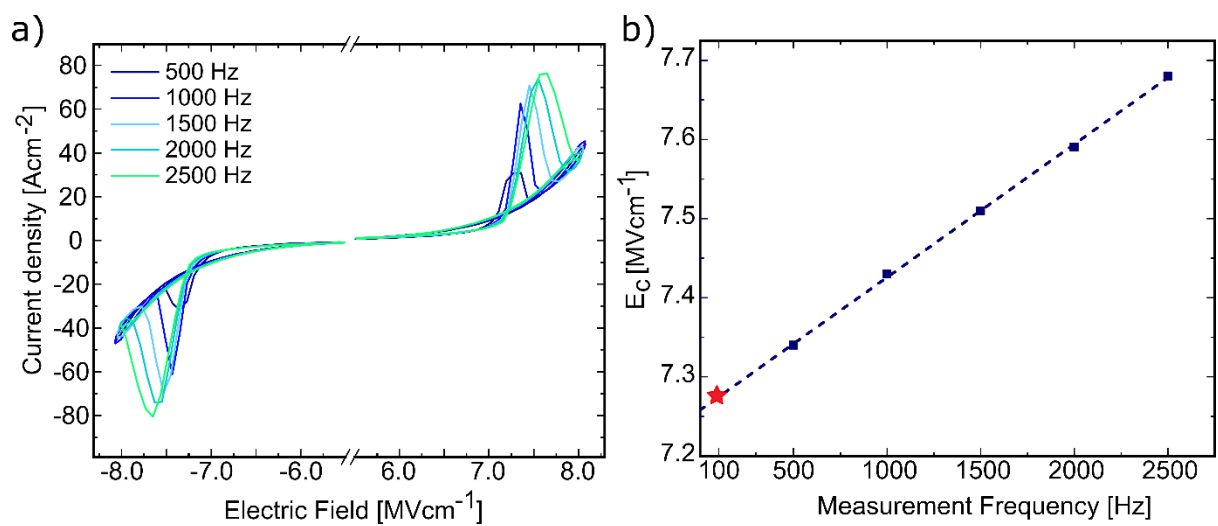

**Figure S7:** a)  $J$ - $E$  measurement at different frequencies. At 100 Hz the leakage in the sample was higher than the current density of the switching peak, making it impossible to extract the coercive field  $E_c$ . b) Therefore  $E_c$  at multiple frequencies was measured and fitted linearly. The extrapolation of the fit is used to extract  $E_c \sim 7.28 \text{ MVcm}^{-1}$  at 100 Hz marked by a red star.

### Composition of AlScBN films via XPS vs Target Power

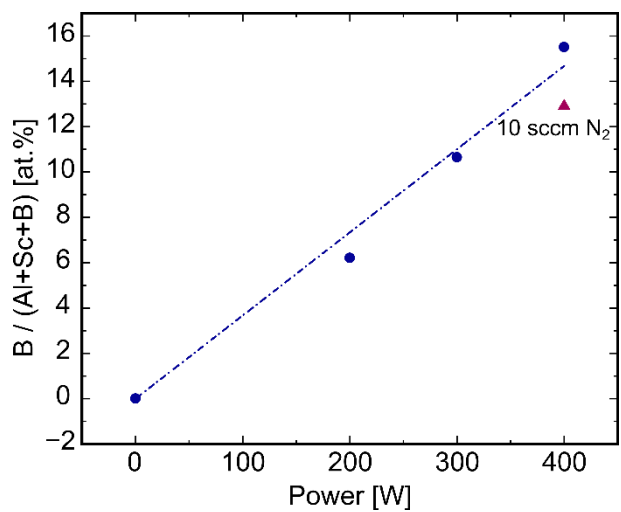

**Figure S8:** Boron concentration determined via XPS over the Power applied to Boron Target during deposition.

## References:

- [1] Martina Baeumler, Yuan Lu, Nicolas Kurz, Lutz Kirste, Mario Prescher, Tim Christoph, Joachim Wagner, Agnė Žukauskaitė, Oliver Ambacher; Optical constants and band gap of wurtzite  $\text{Al}_{1-x}\text{Sc}_x\text{N}/\text{Al}_2\text{O}_3$  prepared by magnetron sputter epitaxy for scandium concentrations up to  $x = 0.41$ . *J. Appl. Phys.* 28 July 2019; 126 (4): 045715. <https://doi.org/10.1063/1.5101043>
- [2] Zanatta, A.R. Revisiting the optical bandgap of semiconductors and the proposal of a unified methodology to its determination. *Sci Rep* 9, 11225 (2019). <https://doi.org/10.1038/s41598-019-47670-y>
